# Supplementary material for: Wide-range optical studies on various single-walled carbon nanotubes: the origin of the low-energy gap
Source: arXiv:1101.4586 ancillary file (2011-06-30)
Supplement: Supplementary file 1 [file PekkerKamarasSuppmat.pdf]

# Wide-range optical studies on various single-walled carbon nanotubes: the origin of the low-energy gap

Á. Pekker*, K. Kamarás
Research Institute for Solid State Physics and Optics, Hungarian Academy of Sciences, P.O. Box 49, H-1525 Budapest, Hungary

SUPPLEMENTAL MATERIAL

This document contains the details of the evaluation of nanotube spectra. For each sample the following information is contained:

1. **Transmission spectrum and optical conductivity (σ).** We calculated σ from the transmission using the Kramers-Kronig relations and the Fresnel equations. We show the optical conductivity also on a logarithmic frequency scale, to emphasize the low-frequency features.

2. **Parameters of the fitted oscillators.** We fitted the optical conductivity using the Drude-Lorentz model. The parameters are: center frequency $\omega_c$ (0 for Drude oscillators), $\omega_p$ plasma frequency, $\gamma$ linewidth. The assignment to specific sets of peaks ($M_{00}$, $S_{11}$, etc.) is indicated by the color code given on each page.

3. **Optical conductivity and the fitted oscillators.**

4. **Extracted peaks.** In order to extract one specific set of peaks ($M_{00}$, $S_{11}$, etc.), the oscillators assigned to other transitions are considered as background and subtracted.

The following information is available only for the undoped tubes:

5. **Wavenumber ranges used in the diameter determination.** The most abundant nanotube types are determined using the first and third quantiles ($Q_1$, $Q_3$) of the background corrected peaks. In the case of the CoMoCat samples the $M_{11}$ peaks are in the visible region and merged into the $\pi$-$\pi^*$ background. In the spectrum, only the contributions from the most abundant metallic nanotubes are detectable. In this case the energy ranges were determined by the parameters of the assigned Lorentzians: $[\omega_{cL} - \gamma_L/2\ ,\ \omega_{cH} + \gamma_H/2]$, where L and H denotes the Lorentzians with the lowest and highest energy respectively. The determined wavenumber ranges were converted to energy and corrected by the 0.07 eV shift due to bundling.

6. **Nanotube species related to the defined regions, and their diameters.**

7. **Average diameters.** Note: the average diameter of non-armchair nanotubes was used in the evaluation of the diameter dependence of the low-frequency gap.

8. **Graphical representation of the most abundant nanotube species.**

* Email addresses: pekkera@szfki.hu, kamaras@szfki.hu

# P2 sample

P2-1. Transmission spectrum and optical conductivity

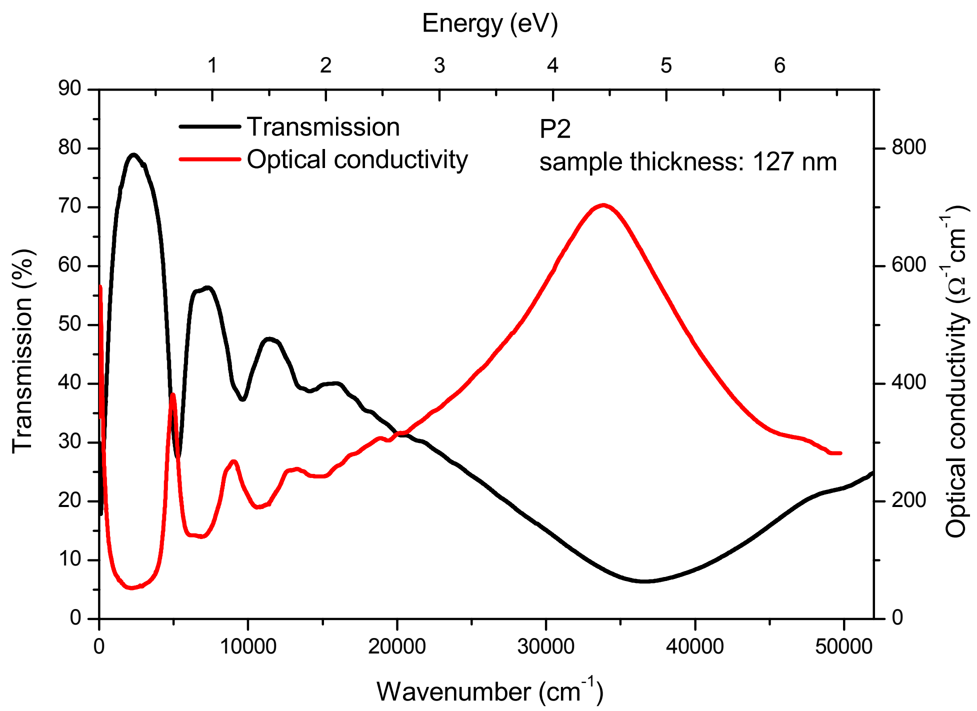


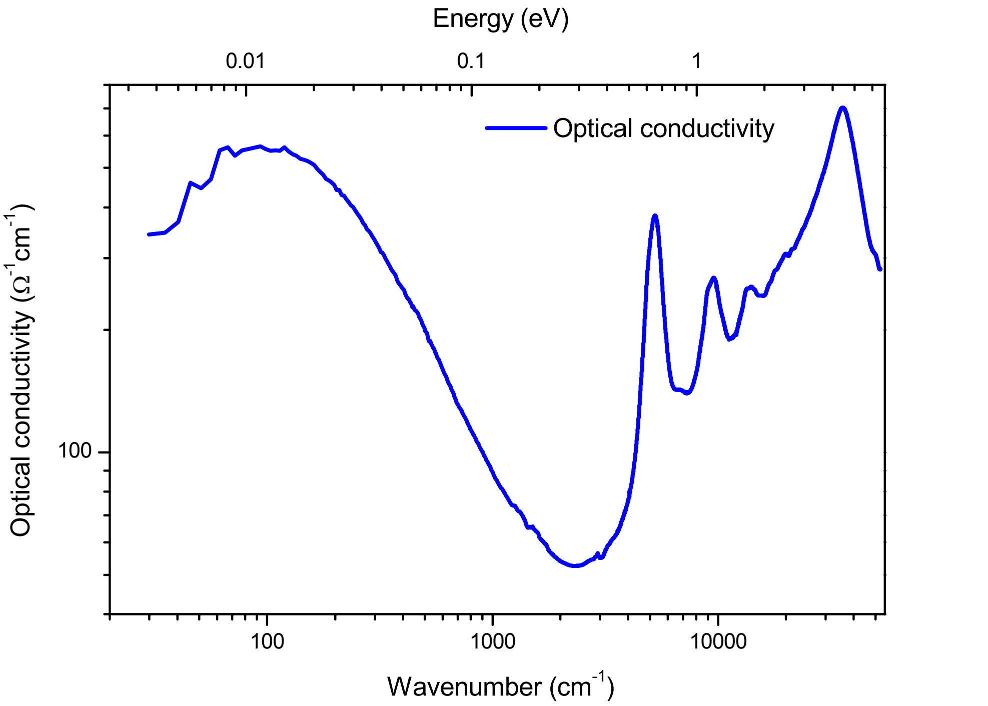

P2-2. Parameters of the Drude-Lorentz fit

| no. | $\omega_c$ (cm$^{-1}$) | $\omega_p$ (cm$^{-1}$) | $\gamma$ (cm$^{-1}$) |
|---|---|---|---|
| 1 | 0 | 912.87 | 122.39 |
| 2 | 0 | 4664.77 | 8925.15 |
| 3 | 109.18 | 3008.04 | 336.44 |
| 4 | 4908.04 | 1759.65 | 562.04 |
| 5 | 5246.15 | 2857.45 | 756.01 |
| 6 | 5409.27 | 2589.54 | 946.03 |
| 7 | 6737.48 | 1447.11 | 1270.04 |
| 8 | 7364.61 | 1596.01 | 1785.39 |
| 9 | 8305.30 | 1750.20 | 1381.69 |
| 10 | 8970.40 | 2137.42 | 960.50 |
| 11 | 9447.19 | 1856.20 | 1056.51 |
| 12 | 9761.61 | 1935.85 | 987.53 |
| 13 | 10411.47 | 2191.64 | 1546.77 |
| 14 | 11686.94 | 758.86 | 1012.19 |
| 15 | 11377.46 | 1882.99 | 2261.45 |
| 16 | 12524.14 | 1629.38 | 1346.43 |
| 17 | 13298.50 | 1971.09 | 1193.68 |
| 18 | 14110.29 | 1800.17 | 1370.85 |
| 19 | 13861.28 | 1023.70 | 1406.14 |
| 20 | 14620.66 | 637.87 | 726.61 |
| 21 | 15346.52 | 2654.19 | 2517.34 |
| 22 | 16802.21 | 1339.73 | 1341.38 |
| 23 | 17681.72 | 638.67 | 901.83 |
| 24 | 17933.50 | 1794.59 | 1841.78 |
| 25 | 18893.65 | 1331.05 | 1353.31 |
| 26 | 19532.79 | 790.66 | 993.87 |
| 27 | 19238.52 | 91.22 | 281.71 |
| 28 | 19998.04 | 1251.95 | 1189.57 |
| 29 | 21186.35 | 906.85 | 977.98 |
| 30 | 22472.19 | 675.58 | 1224.92 |
| 31 | 23510.54 | 468.27 | 814.59 |
| 32 | 30444.96 | 27361.14 | 37394.03 |
| 33 | 35552.49 | 1775.99 | 3254.01 |
| 34 | 36199.12 | 16529.94 | 12228.59 |
| 35 | 51138.57 | 3045.19 | 4318.07 |

- $M_{00}$
- $S_{11}$
- $S_{22}$
- $M_{11}$
- $M_{22} + S_{33}$
- Background

P2-3. Optical conductivity and the fitted oscillators

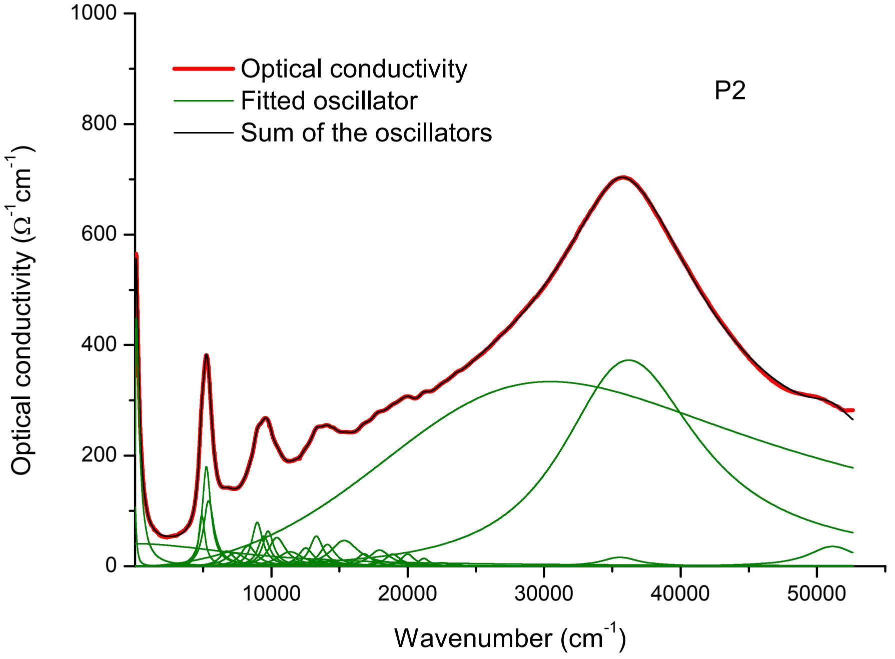


P2-4. The extracted $M_{00}$, $S_{11}$, $S_{22}$, $M_{11}$, etc. peaks

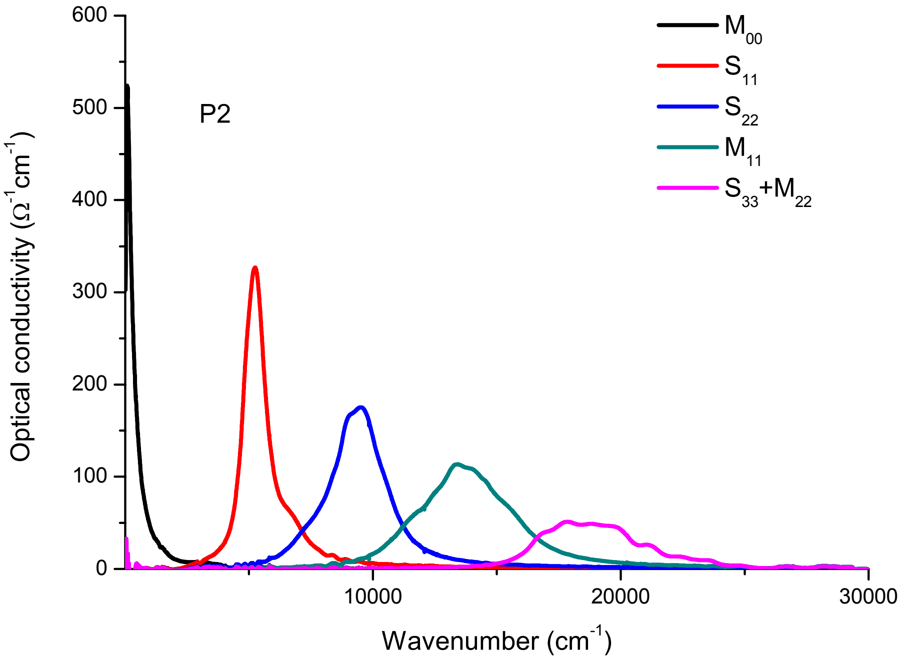

P2-5. The wavenumber ranges used in the diameter determination

| Wavenumber ranges for diameter determination | | | |
|---|---|---|---|
| Semiconducting | 4880 | - | 5811 |
| Metallic | 12072 | - | 14970 |

P2-6. Semiconducting and metallic nanotube species with transitions in the defined regions

| $S_{11}$ (eV) | n | m | d (nm) |
|---|---|---|---|
| 0.779 | 15 | 4 | 1.377 |
| 0.764 | 11 | 9 | 1.377 |
| 0.762 | 15 | 2 | 1.278 |
| 0.759 | 14 | 4 | 1.300 |
| 0.757 | 14 | 6 | 1.411 |
| 0.752 | 13 | 6 | 1.336 |
| 0.740 | 12 | 8 | 1.384 |
| 0.735 | 18 | 1 | 1.470 |
| 0.729 | 13 | 8 | 1.457 |
| 0.727 | 17 | 3 | 1.483 |
| 0.723 | 11 | 10 | 1.444 |
| 0.712 | 16 | 5 | 1.508 |
| 0.707 | 17 | 1 | 1.391 |
| 0.705 | 16 | 3 | 1.405 |
| 0.700 | 15 | 5 | 1.431 |
| 0.697 | 12 | 10 | 1.515 |
| 0.692 | 14 | 7 | 1.470 |
| 0.692 | 15 | 7 | 1.546 |
| 0.680 | 13 | 9 | 1.521 |

| $M_{11}$ (eV) | n | m | d (nm) |
|---|---|---|---|
| 1.918 | 9 | 9 | 1.238 |
| 1.910 | 12 | 6 | 1.260 |
| 1.891 | 16 | 1 | 1.312 |
| 1.862 | 15 | 3 | 1.326 |
| 1.831 | 11 | 8 | 1.312 |
| 1.810 | 14 | 5 | 1.354 |
| 1.754 | 10 | 10 | 1.375 |
| 1.754 | 18 | 0 | 1.429 |
| 1.746 | 13 | 7 | 1.396 |
| 1.742 | 17 | 2 | 1.436 |
| 1.709 | 16 | 4 | 1.455 |
| 1.679 | 12 | 9 | 1.449 |
| 1.661 | 15 | 6 | 1.487 |
| 1.614 | 11 | 11 | 1.513 |
| 1.610 | 18 | 3 | 1.562 |
| 1.606 | 14 | 8 | 1.531 |
| 1.577 | 17 | 5 | 1.586 |

P2-7. The calculated average diameters

| average diameter (nm) | |
|---|---|
| semiconducting | 1.426 |
| metallic | 1.413 |
| overall | 1.420 |
| non armchair metallic | 1.421 |

P2-8. The most abundant nanotubes in the sample

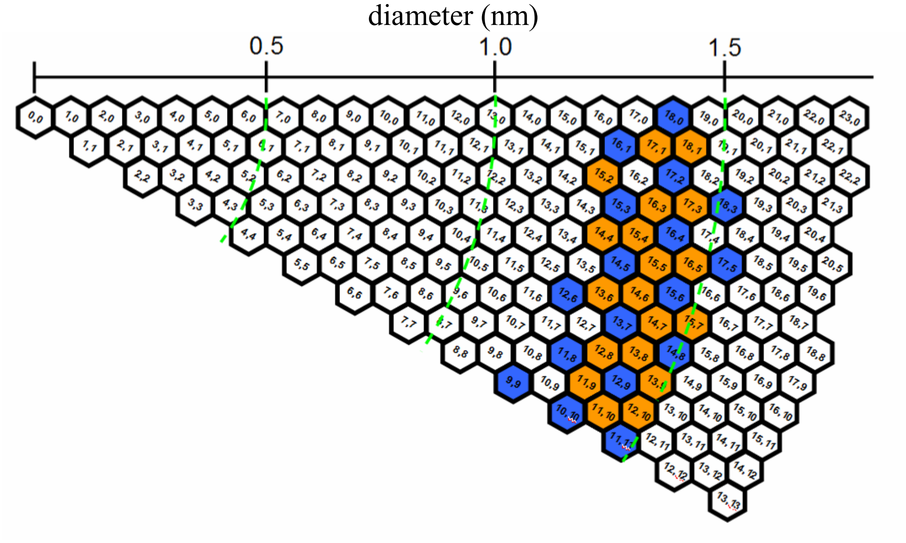


metallic and small-gap nanotube

semiconducting nanotube

# P3 sample

P3-1. Transmission spectrum and optical conductivity

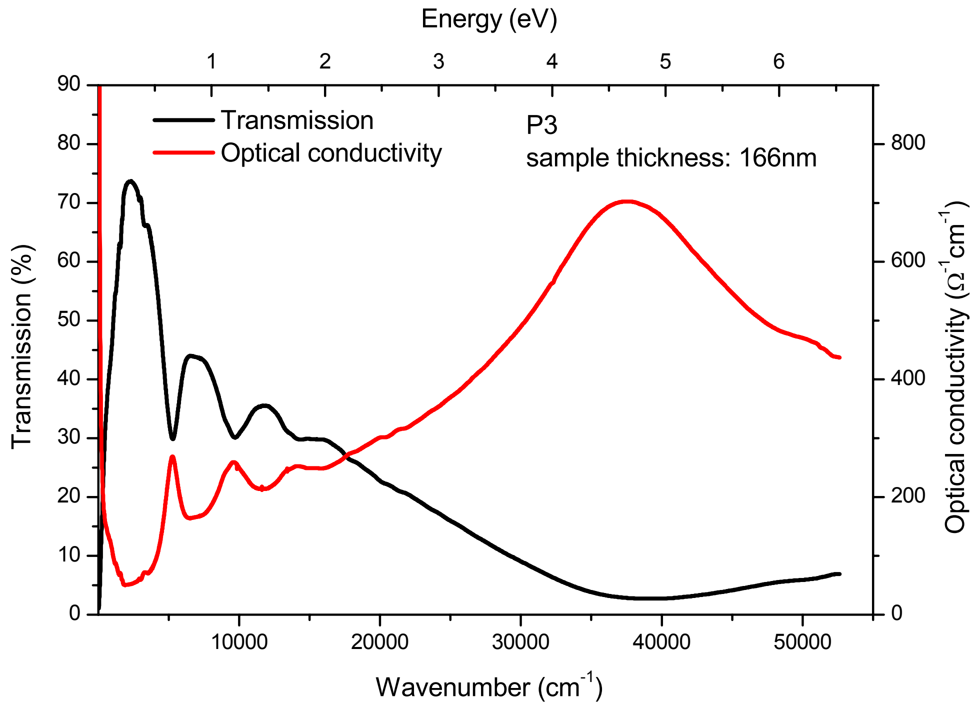


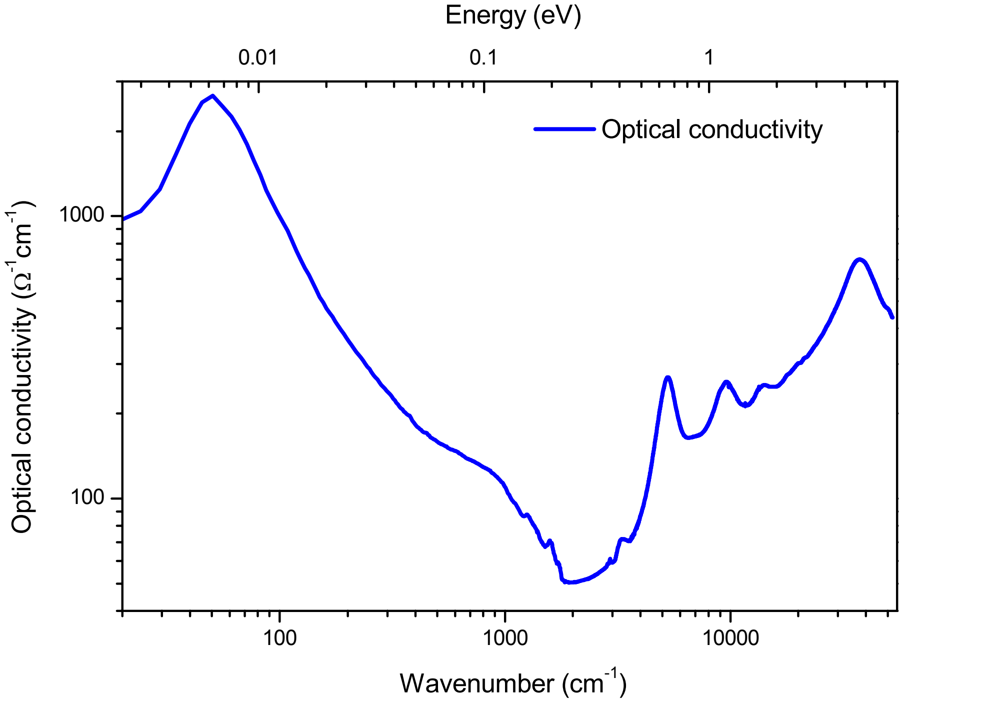

P3-2. Parameters of the Drude-Lorentz fit

| no. | $\omega_c$ ($cm^{-1}$) | $\omega_p$ ($cm^{-1}$) | $\gamma$ ($cm^{-1}$) |
|---|---|---|---|
| 1 | 0 | 2843.68 | 919.47 |
| 2 | 0 | 5119.54 | 17158.52 |
| 3 | 49.47 | 2815.87 | 55.87 |
| 4 | 5030.47 | 2060.45 | 1444.15 |
| 5 | 5281.18 | 2537.70 | 1018.90 |
| 6 | 5348.79 | 2235.41 | 1626.94 |
| 7 | 6879.98 | 2006.69 | 1848.95 |
| 8 | 8161.76 | 2347.00 | 2332.89 |
| 9 | 8888.00 | 1384.98 | 1153.87 |
| 10 | 9334.38 | 1873.54 | 2100.22 |
| 11 | 9675.38 | 2618.39 | 1613.80 |
| 12 | 10517.89 | 1654.13 | 1493.25 |
| 13 | 11524.07 | 1536.96 | 1848.86 |
| 14 | 12448.56 | 1168.45 | 1745.29 |
| 15 | 12849.49 | 354.78 | 1047.63 |
| 16 | 13229.72 | 524.99 | 762.82 |
| 17 | 13452.65 | 1741.21 | 1935.54 |
| 18 | 14096.60 | 338.95 | 615.86 |
| 19 | 14352.83 | 2148.29 | 2387.29 |
| 20 | 15332.32 | 418.71 | 1773.76 |
| 21 | 15455.62 | 779.80 | 1430.99 |
| 22 | 16821.69 | 1145.05 | 2375.76 |
| 23 | 17848.31 | 859.11 | 1218.96 |
| 24 | 18853.58 | 763.86 | 1358.81 |
| 25 | 19716.79 | 887.10 | 1389.93 |
| 26 | 20079.59 | 336.18 | 646.38 |
| 27 | 21201.01 | 476.16 | 662.89 |
| 28 | 27473.58 | 26060.32 | 44901.15 |
| 29 | 27731.00 | 727.07 | 2780.18 |
| 30 | 37902.58 | 21852.20 | 17423.93 |
| 31 | 53006.36 | 11823.29 | 16502.12 |

$M_{00}$

$S_{11}$

$S_{22}$

$M_{11}$

$M_{22}$ + $S_{33}$

Background

P3-3. Optical conductivity and the fitted oscillators

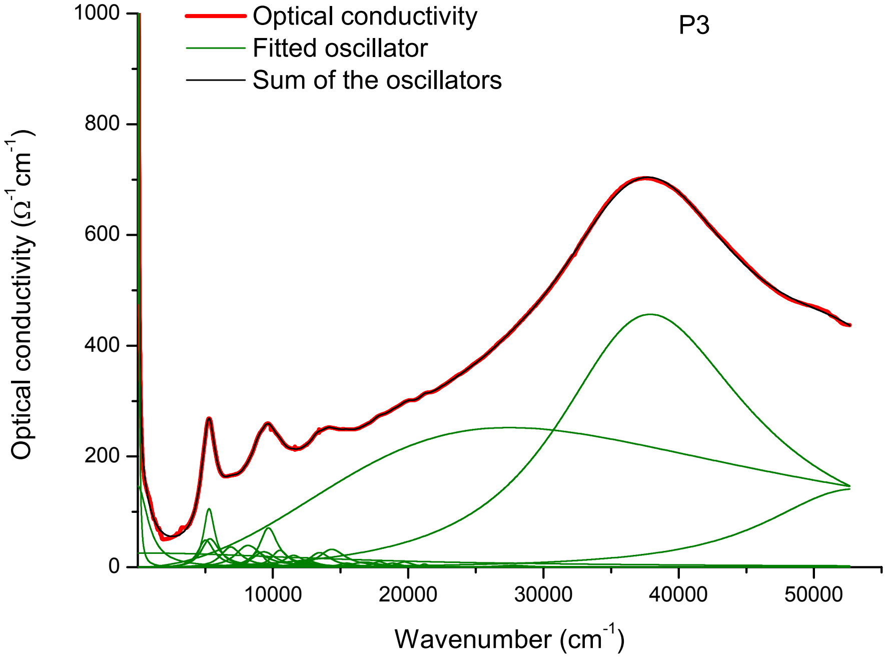


P3-4. The extracted $M_{00}$, $S_{11}$, $S_{22}$, $M_{11}$, etc. peaks

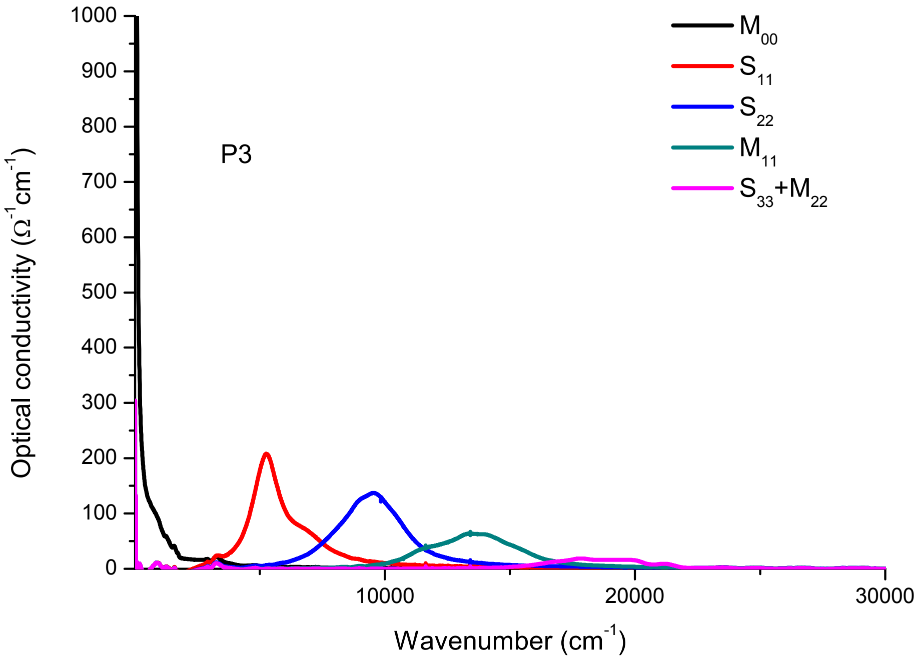


We considered that **P3** has the same diameter distribution as the **P2** sample (see data at the manufacturer's homepage: www.carbonsolution.com).

# Laser - H sample

Laser-H-1. Transmission spectrum and optical conductivity

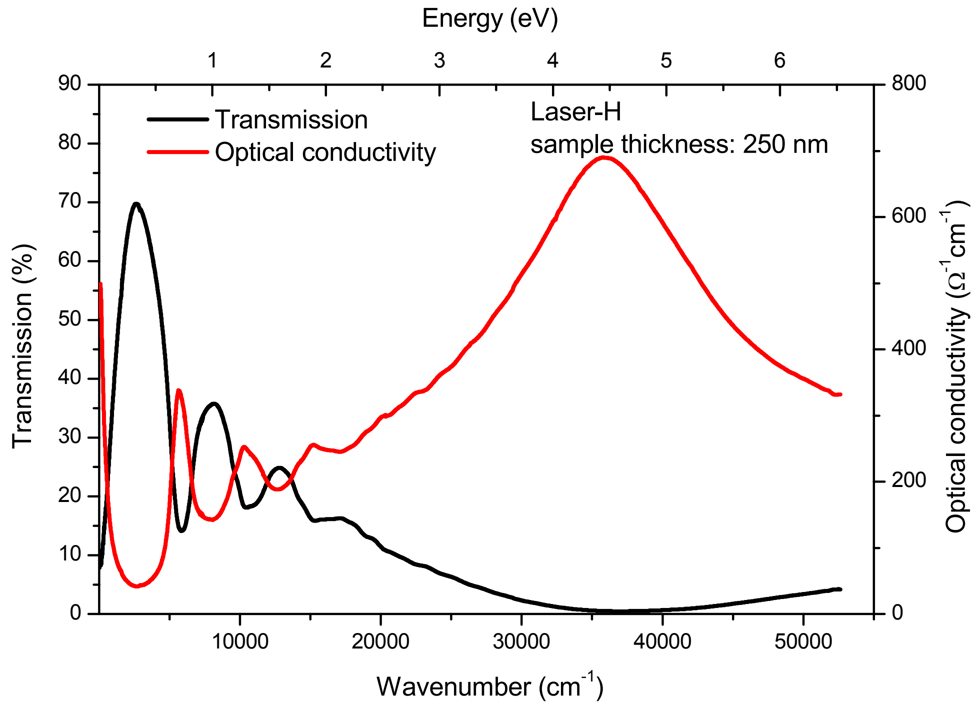


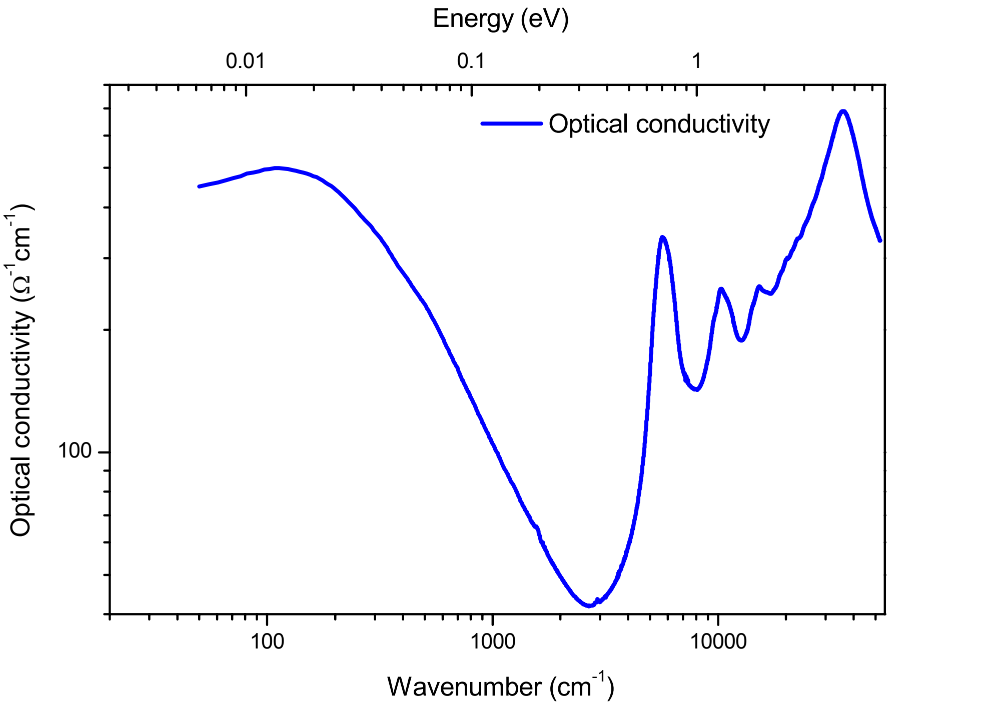

Laser-H-2. Parameters of the Drude-Lorentz fit

| no. | $\omega_c$ ($cm^{-1}$) | $\omega_p$ ($cm^{-1}$) | $\gamma$ ($cm^{-1}$) |
|---|---|---|---|
| 1 | 0 | 2860.01 | 677.94 |
| 2 | 0 | 3672.86 | 12784.25 |
| 3 | 113.64 | 2252.22 | 294.35 |
| 4 | 5279.64 | 1677.75 | 663.25 |
| 5 | 5636.09 | 2822.00 | 797.69 |
| 6 | 5784.60 | 1495.97 | 3055.69 |
| 7 | 6123.37 | 2837.02 | 994.25 |
| 8 | 7697.80 | 2919.25 | 3438.45 |
| 9 | 9516.67 | 1731.66 | 1299.72 |
| 10 | 10245.78 | 1448.94 | 895.23 |
| 11 | 10402.50 | 2519.23 | 2356.50 |
| 12 | 11141.38 | 2891.14 | 2181.15 |
| 13 | 12726.89 | 43.28 | 146.72 |
| 14 | 14173.23 | 1809.07 | 2087.64 |
| 15 | 15068.55 | 1832.85 | 1918.32 |
| 16 | 15177.16 | 567.48 | 695.60 |
| 17 | 16067.54 | 2022.53 | 2792.89 |
| 18 | 18576.79 | 178.62 | 2238.12 |
| 19 | 18876.11 | 604.15 | 766.85 |
| 20 | 20008.50 | 1128.80 | 1482.04 |
| 21 | 21352.77 | 540.70 | 1116.77 |
| 22 | 22320.17 | 664.22 | 967.04 |
| 23 | 27394.57 | 24248.80 | 37086.34 |
| 24 | 36265.60 | 19446.55 | 14821.10 |
| 25 | 58537.74 | 15920.59 | 35788.69 |

- $M_{00}$
- $S_{11}$
- $S_{22}$
- $M_{11}$
- $M_{22}$ + $S_{33}$
- Background

Laser-H-3. Optical conductivity and the fitted oscillators

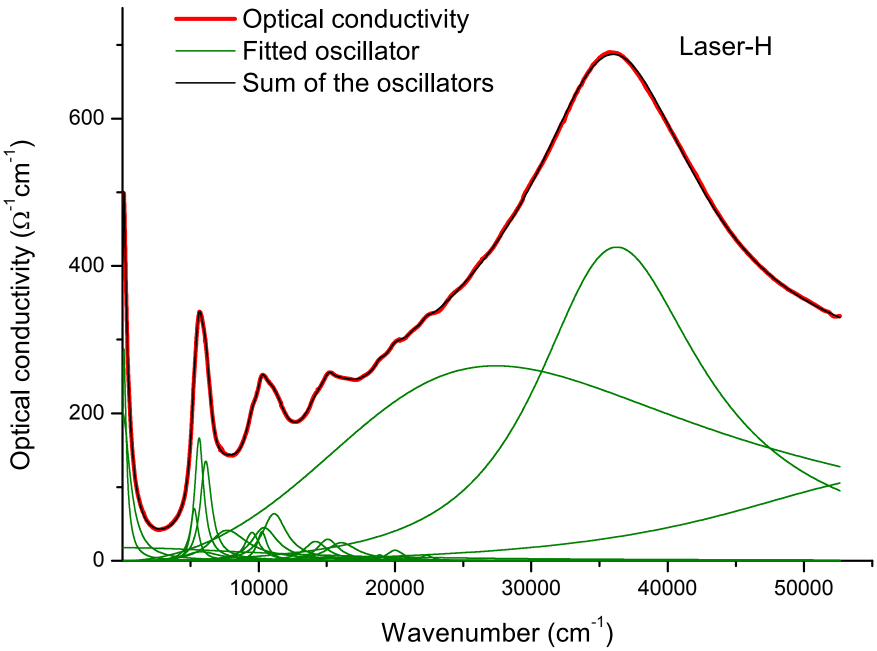


Laser-H-4. The extracted $M_{00}$, $S_{11}$, $S_{22}$, $M_{11}$, etc. peaks

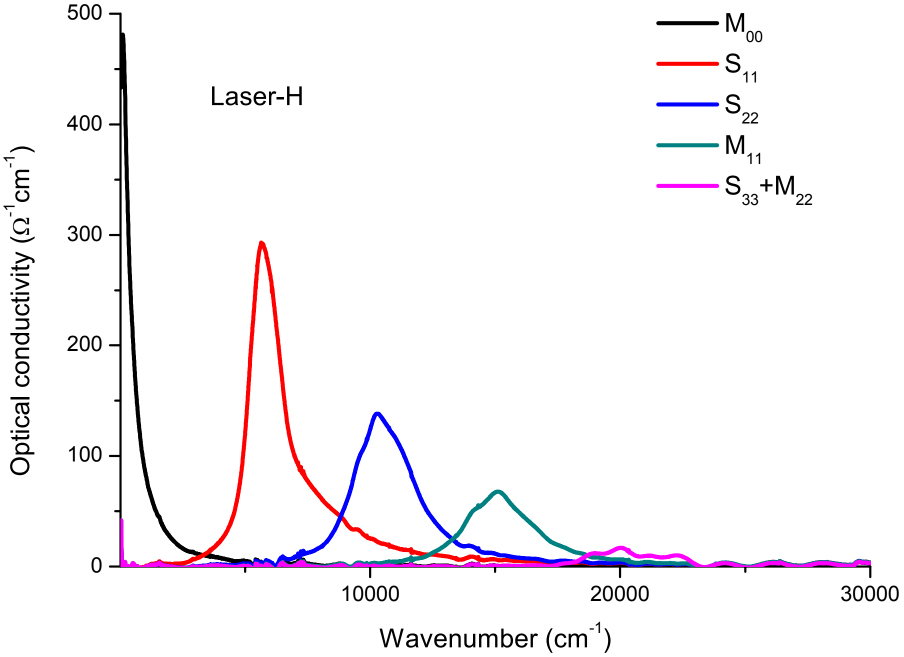

Laser-H-5. The wavenumber ranges used in the diameter determination

| Wavenumber ranges for diameter determination | | | |
|---|---|---|---|
| Semiconducting | 5330 | - | 6897 |
| Metallic | 13901 | - | 16373 |

Laser-H-6. Semiconducting and metallic nanotube species with transitions in the defined regions

| $S_{11}$ (eV) | n | m | d (nm) |
|---|---|---|---|
| 0.926 | 12 | 4 | 1.145 |
| 0.903 | 12 | 2 | 1.041 |
| 0.903 | 11 | 4 | 1.068 |
| 0.902 | 13 | 0 | 1.032 |
| 0.896 | 10 | 6 | 1.111 |
| 0.889 | 11 | 6 | 1.186 |
| 0.879 | 9 | 8 | 1.170 |
| 0.871 | 15 | 1 | 1.232 |
| 0.858 | 14 | 3 | 1.248 |
| 0.844 | 10 | 8 | 1.240 |
| 0.833 | 13 | 5 | 1.278 |
| 0.828 | 14 | 1 | 1.153 |
| 0.827 | 13 | 3 | 1.170 |
| 0.822 | 12 | 5 | 1.201 |
| 0.812 | 11 | 7 | 1.248 |
| 0.801 | 12 | 7 | 1.321 |
| 0.794 | 10 | 9 | 1.307 |
| 0.793 | 16 | 2 | 1.357 |
| 0.779 | 15 | 4 | 1.377 |
| 0.764 | 11 | 9 | 1.377 |
| 0.762 | 15 | 2 | 1.278 |
| 0.759 | 14 | 4 | 1.300 |
| 0.757 | 14 | 6 | 1.411 |
| 0.752 | 13 | 6 | 1.336 |
| 0.740 | 12 | 8 | 1.384 |
| 0.735 | 18 | 1 | 1.470 |

| $M_{11}$ (eV) | n | m | d (nm) |
|---|---|---|---|
| 2.104 | 11 | 5 | 1.126 |
| 2.059 | 15 | 0 | 1.191 |
| 2.039 | 14 | 2 | 1.199 |
| 2.009 | 10 | 7 | 1.175 |
| 1.984 | 13 | 4 | 1.222 |
| 1.918 | 9 | 9 | 1.238 |
| 1.910 | 12 | 6 | 1.260 |
| 1.891 | 16 | 1 | 1.312 |
| 1.862 | 15 | 3 | 1.326 |
| 1.831 | 11 | 8 | 1.312 |
| 1.810 | 14 | 5 | 1.354 |

Laser-H-7. The calculated average diameters

| average diameter (nm) | |
|---|---|
| semiconducting | 1.247 |
| metallic | 1.246 |
| overall | 1.247 |
| non armchair metallic | 1.247 |

Laser-H-8. The most abundant nanotubes in the sample

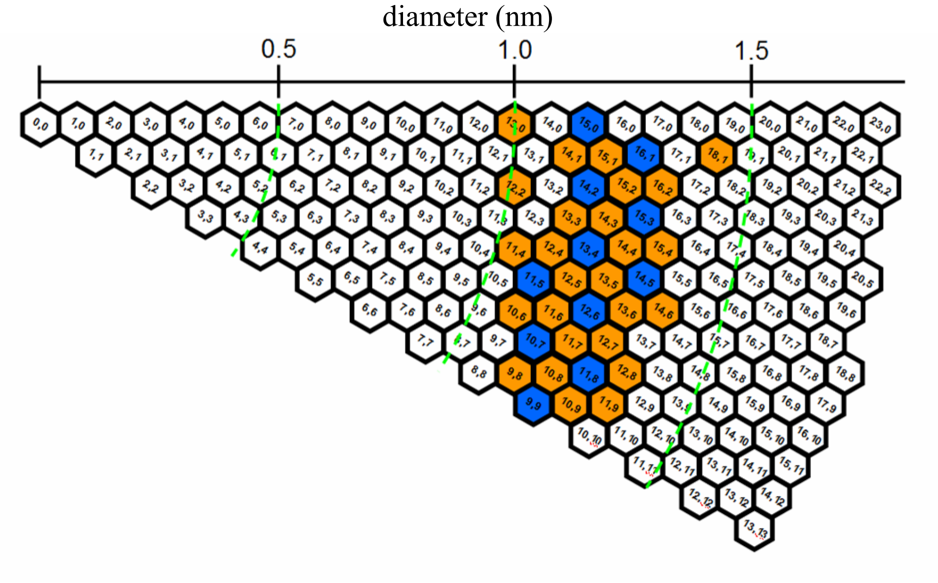


metallic and small-gap nanotube

semiconducting nanotube

# Laser sample

Laser-1. Transmission spectrum and optical conductivity

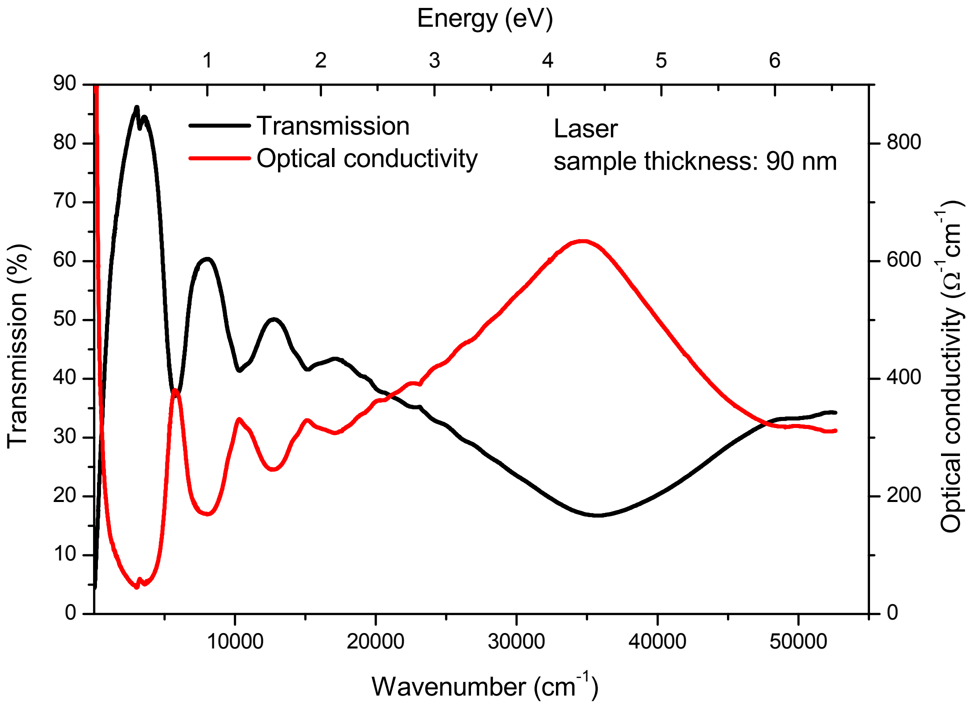


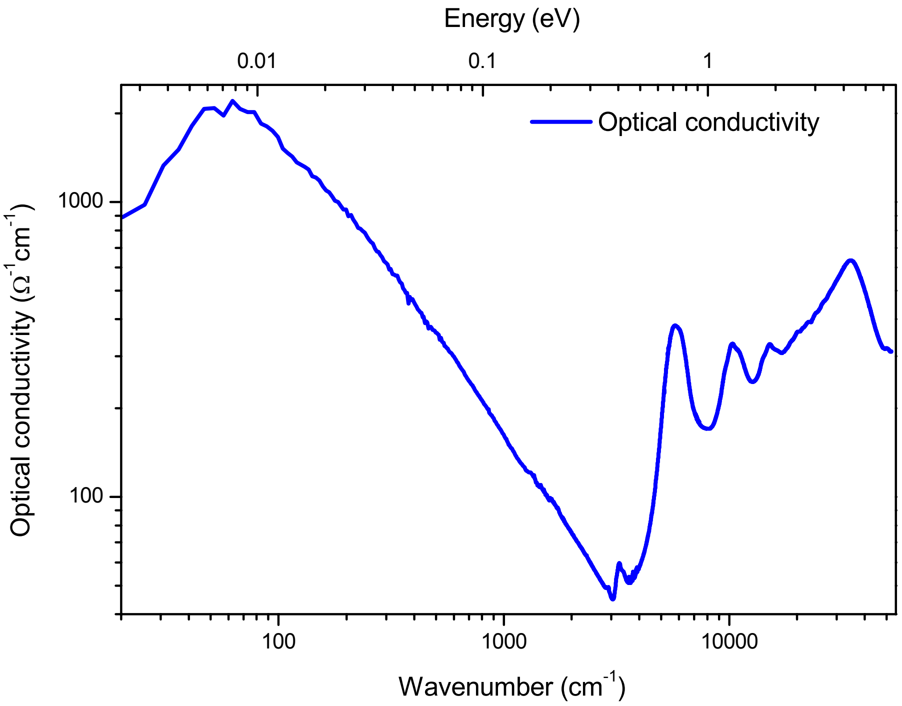

Laser-2. Parameters of the Drude-Lorentz fit

| no. | $\omega_c$ ($cm^{-1}$) | $\omega_p$ ($cm^{-1}$) | $\gamma$ ($cm^{-1}$) |
|---|---|---|---|
| 1 | 0 | 3606.74 | 377.86 |
| 2 | 0 | 3246.40 | 1799.59 |
| 3 | 61.75 | 2992.44 | 107.61 |
| 4 | 5212.01 | 1653.77 | 685.86 |
| 5 | 5542.90 | 2479.65 | 745.60 |
| 6 | 5832.15 | 2236.08 | 842.12 |
| 7 | 6202.39 | 3375.54 | 1117.03 |
| 8 | 7611.78 | 2901.03 | 2568.52 |
| 9 | 9594.98 | 2653.75 | 1549.42 |
| 10 | 10171.53 | 352.97 | 448.14 |
| 11 | 10259.36 | 1870.93 | 985.05 |
| 12 | 10800.47 | 3376.15 | 2546.96 |
| 13 | 11180.21 | 3010.47 | 2121.53 |
| 14 | 12834.64 | 1513.37 | 2229.95 |
| 15 | 14160.04 | 2278.91 | 1620.59 |
| 16 | 14985.70 | 1361.06 | 1099.88 |
| 17 | 15288.63 | 1973.48 | 1619.41 |
| 18 | 16265.62 | 2039.74 | 1993.61 |
| 19 | 18127.81 | 1457.41 | 2367.26 |
| 20 | 18878.82 | 610.16 | 753.96 |
| 21 | 19970.67 | 1170.91 | 1253.65 |
| 22 | 21439.97 | 927.45 | 1857.25 |
| 23 | 25642.51 | 24706.75 | 31557.14 |
| 24 | 35345.37 | 18212.15 | 15327.81 |
| 25 | 61682.11 | 17262.33 | 12948.42 |

$M_{00}$

$S_{11}$

$S_{22}$

$M_{11}$

$M_{22} + S_{33}$

Background

Laser-3. Optical conductivity and the fitted oscillators

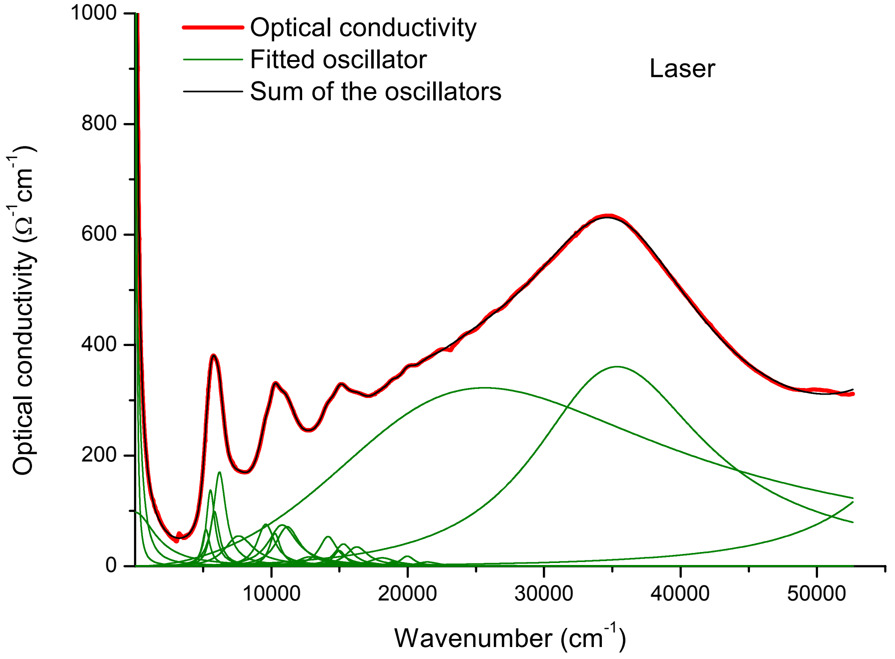


Laser-4. The extracted $M_{00}$, $S_{11}$, $S_{22}$, $M_{11}$, etc. peaks

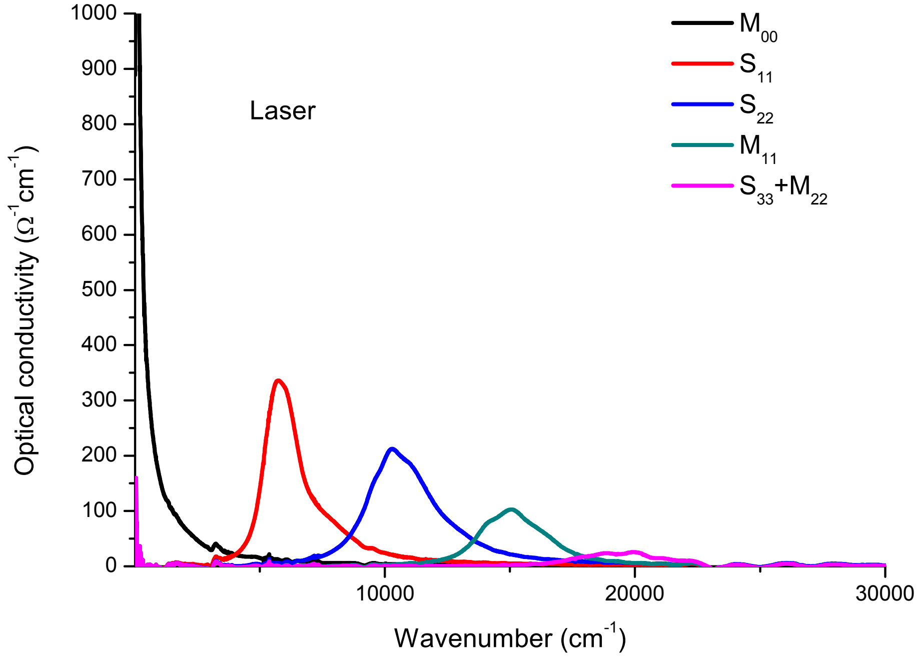


We considered that **Laser** has the same diameter distribution as the **Laser-H** sample, since the latter was obtained by annealing the former.

# HiPco sample

HiPco-1. Transmission spectrum and optical conductivity

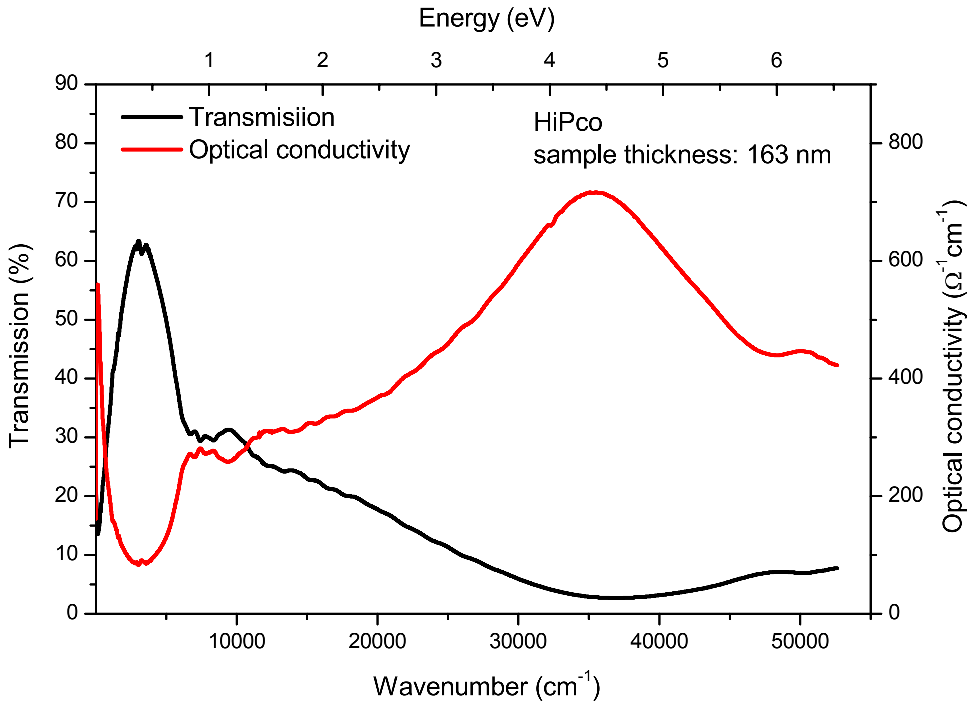


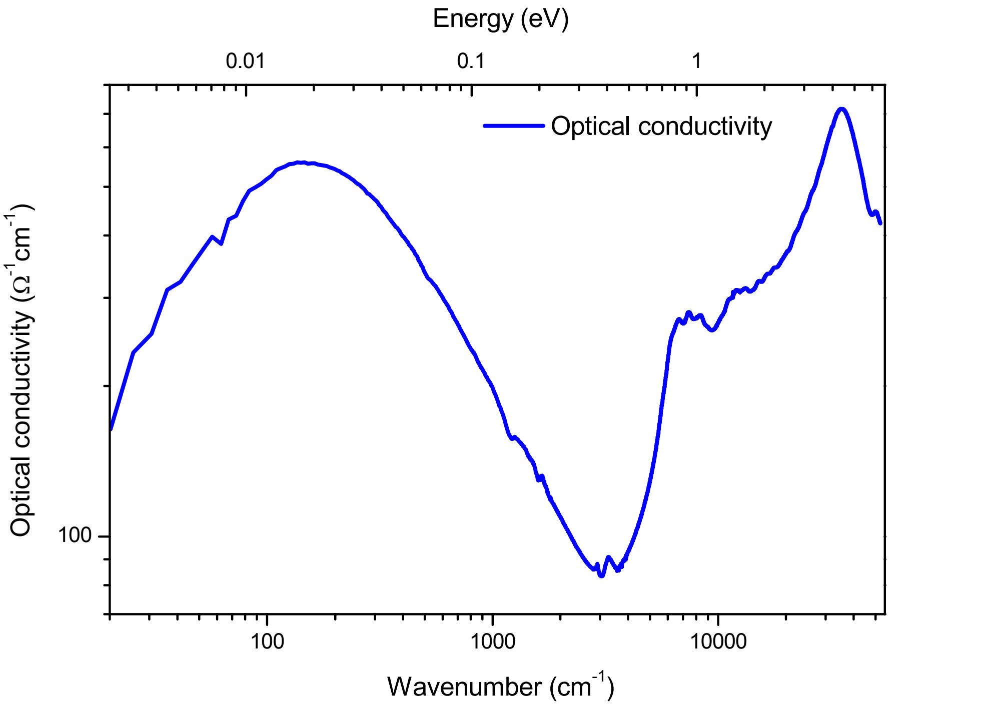

HiPco-2. Parameters of the Drude-Lorentz fit

| no. | $\omega_c$ ($cm^{-1}$) | $\omega_p$ ($cm^{-1}$) | $\gamma$ ($cm^{-1}$) |
|---|---|---|---|
| 1 | 0 | 5126.72 | 12159.54 |
| 2 | 0 | 3494.28 | 1594.35 |
| 3 | 154.69 | 3235.71 | 446.99 |
| 4 | 4574.07 | 1373.81 | 1902.08 |
| 5 | 5666.69 | 2196.64 | 1553.56 |
| 6 | 6192.33 | 2011.29 | 941.86 |
| 7 | 6710.79 | 2204.52 | 954.47 |
| 8 | 7410.06 | 2384.62 | 1033.73 |
| 9 | 8022.01 | 1609.64 | 1015.48 |
| 10 | 8391.69 | 877.19 | 621.39 |
| 11 | 8862.77 | 3563.70 | 2261.94 |
| 12 | 10279.13 | 3174.48 | 2204.27 |
| 13 | 11083.71 | 1461.72 | 1041.60 |
| 14 | 11956.18 | 3093.47 | 1873.25 |
| 15 | 12651.10 | 873.16 | 1211.19 |
| 16 | 13261.32 | 2644.56 | 1901.44 |
| 17 | 14300.51 | 2336.18 | 2211.32 |
| 18 | 15111.89 | 1677.61 | 1420.31 |
| 19 | 15868.28 | 1656.12 | 2111.96 |
| 20 | 16401.71 | 1407.53 | 1420.37 |
| 21 | 17580.28 | 2657.25 | 2661.70 |
| 22 | 19320.08 | 1599.21 | 2196.02 |
| 23 | 20156.92 | 580.86 | 941.60 |
| 24 | 21828.04 | 1331.22 | 1947.45 |
| 25 | 23708.20 | 683.85 | 1040.75 |
| 26 | 25808.03 | 423.72 | 637.67 |
| 27 | 29083.81 | 28592.97 | 36565.84 |
| 28 | 35627.50 | 17246.71 | 14609.67 |
| 29 | 42408.09 | 7196.89 | 12277.39 |
| 30 | 51606.15 | 7879.52 | 7457.76 |

$M_{00}$

$S_{11}$

$S_{22}$

$M_{11}$

$S_{33}$

Background

HiPco-3. Optical conductivity and the fitted oscillators

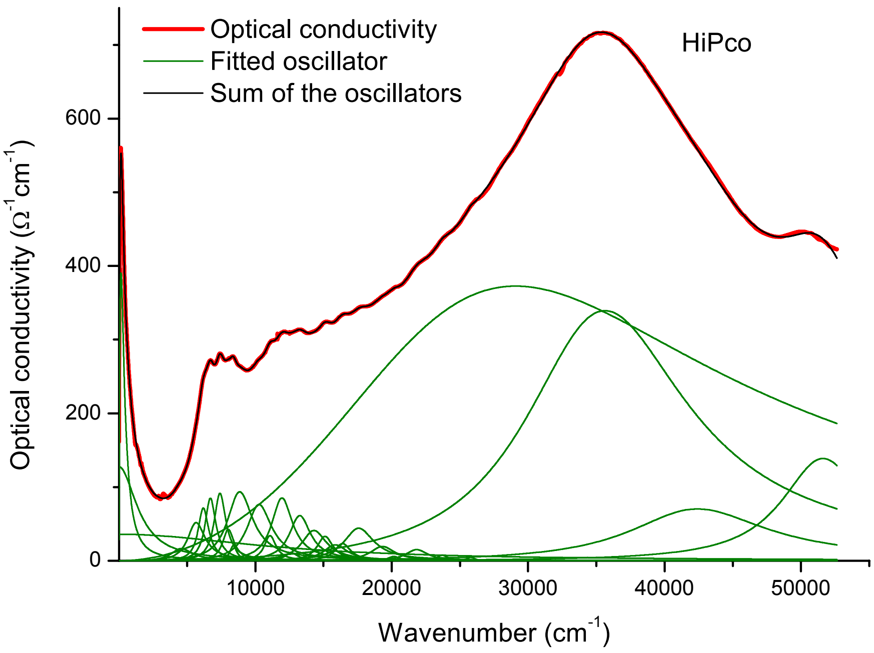


HiPco-4. The extracted $M_{00}$, $S_{11}$, $S_{22}$, $M_{11}$, etc. peaks

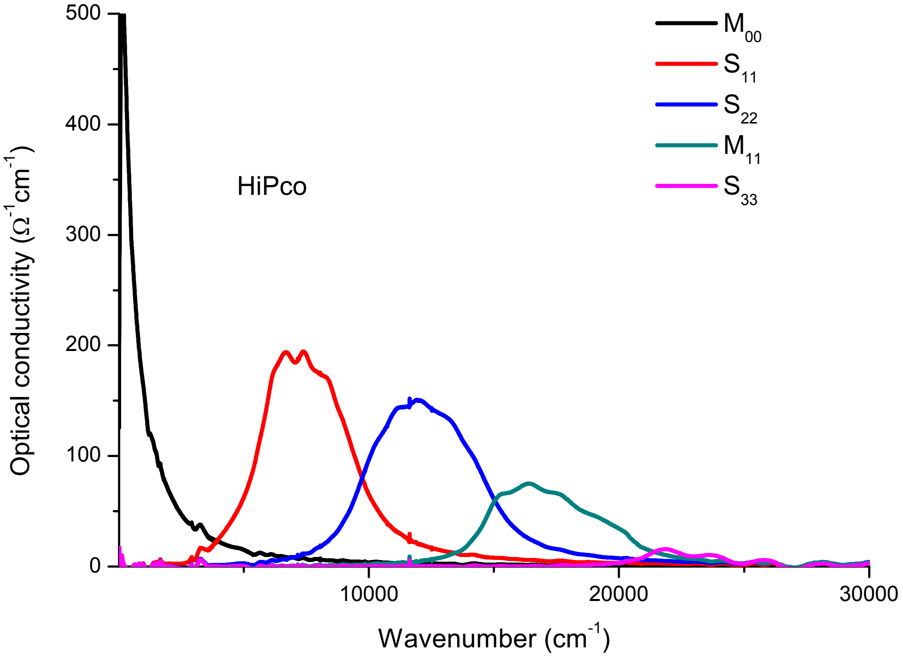

HiPco-5. The wavenumber ranges used in the diameter determination

| Wavenumber ranges for diameter determination | | | |
|---|---|---|---|
| Semiconducting | 5924 | - | 8440 |
| Metallic | 15317 | - | 18612 |

HiPco-6. Semiconducting and metallic nanotube species with transitions in the defined regions

| $S_{11}$ (eV) | n | m | d (nm) |
|---|---|---|---|
| 1.113 | 8 | 4 | 0.840 |
| 1.112 | 7 | 6 | 0.895 |
| 1.095 | 9 | 2 | 0.806 |
| 1.083 | 10 | 0 | 0.794 |
| 1.064 | 8 | 6 | 0.966 |
| 1.062 | 12 | 1 | 0.995 |
| 1.039 | 11 | 3 | 1.014 |
| 0.996 | 9 | 5 | 0.976 |
| 0.996 | 10 | 5 | 1.050 |
| 0.995 | 10 | 3 | 0.936 |
| 0.989 | 11 | 1 | 0.916 |
| 0.983 | 8 | 7 | 1.032 |
| 0.951 | 13 | 2 | 1.120 |
| 0.942 | 9 | 7 | 1.103 |
| 0.926 | 12 | 4 | 1.145 |
| 0.903 | 12 | 2 | 1.041 |
| 0.903 | 11 | 4 | 1.068 |
| 0.902 | 13 | 0 | 1.032 |
| 0.896 | 10 | 6 | 1.111 |
| 0.889 | 11 | 6 | 1.186 |
| 0.879 | 9 | 8 | 1.170 |
| 0.871 | 15 | 1 | 1.232 |
| 0.858 | 14 | 3 | 1.248 |
| 0.844 | 10 | 8 | 1.240 |
| 0.833 | 13 | 5 | 1.278 |
| 0.828 | 14 | 1 | 1.153 |
| 0.827 | 13 | 3 | 1.170 |
| 0.822 | 12 | 5 | 1.201 |
| 0.812 | 11 | 7 | 1.248 |

| $M_{11}$ (eV) | n | m | d (nm) |
|---|---|---|---|
| 2.339 | 7 | 7 | 0.963 |
| 2.336 | 10 | 4 | 0.992 |
| 2.243 | 13 | 1 | 1.074 |
| 2.220 | 9 | 6 | 1.038 |
| 2.190 | 12 | 3 | 1.091 |
| 2.111 | 8 | 8 | 1.100 |
| 2.104 | 11 | 5 | 1.126 |
| 2.059 | 15 | 0 | 1.191 |
| 2.039 | 14 | 2 | 1.199 |
| 2.009 | 10 | 7 | 1.175 |
| 1.984 | 13 | 4 | 1.222 |

HiPco-7. The calculated average diameters

| average diameter (nm) | |
|---|---|
| semiconducting | 1.067 |
| metallic | 1.106 |
| overall | 1.078 |
| non armchair metallic | 1.123 |

HiPco-8. The most abundant nanotubes in the sample

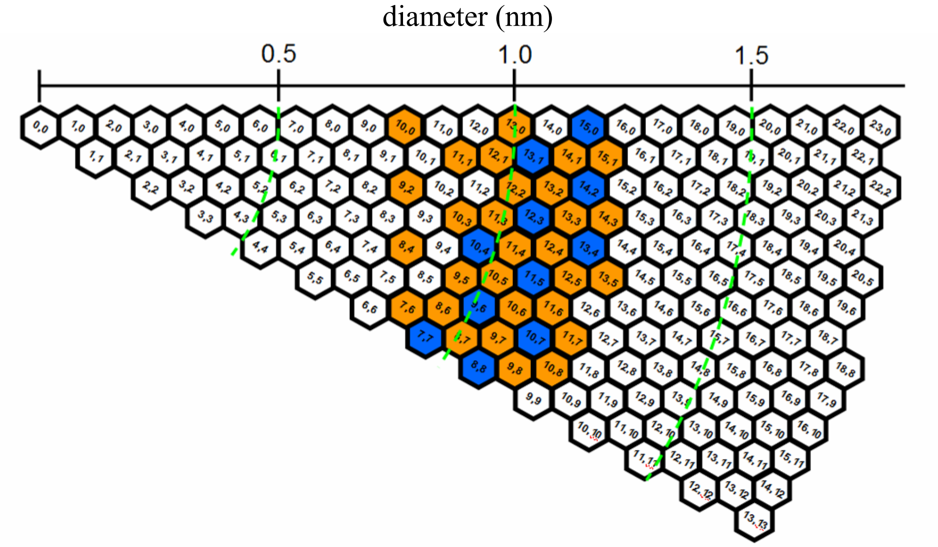


metallic and small-gap nanotube

semiconducting nanotube

# CoMoCat CG sample

CG-1. Transmission spectrum and optical conductivity

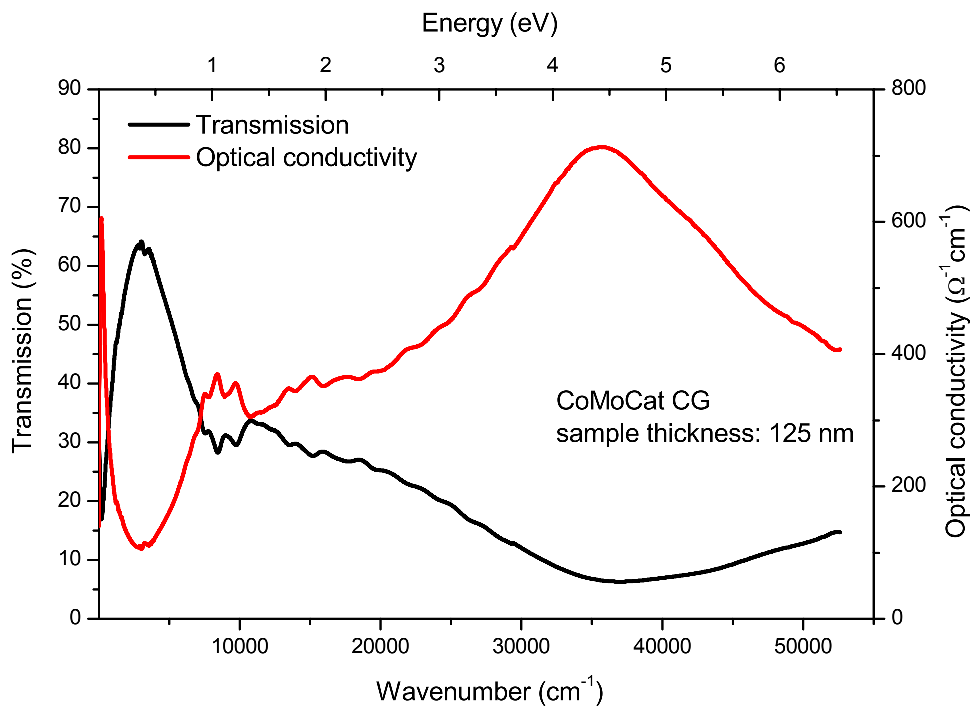


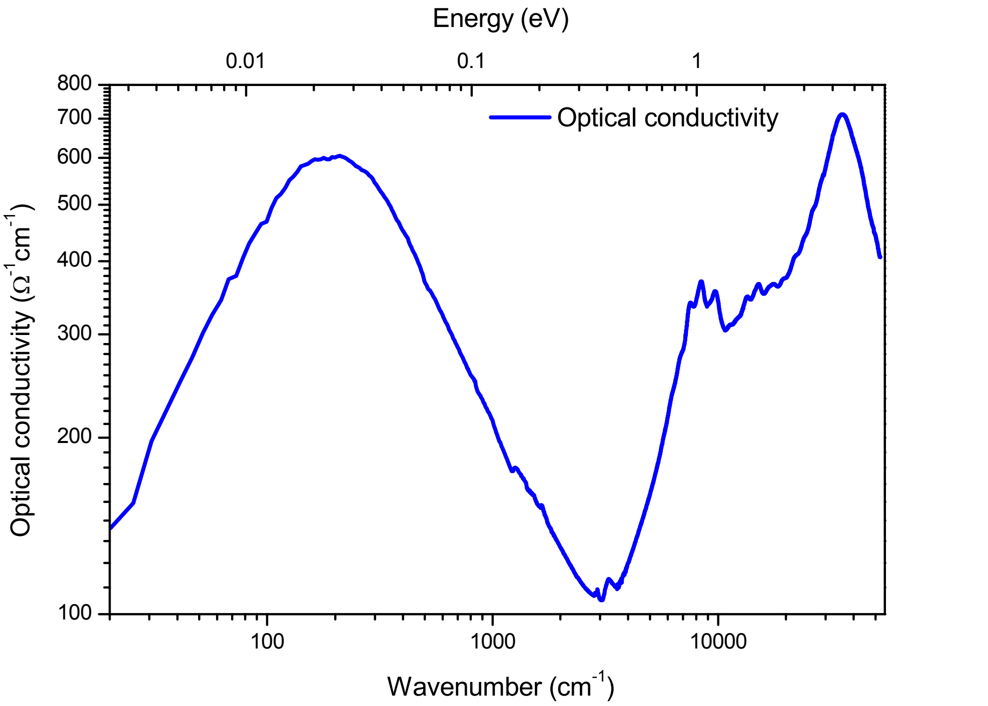

CG-2. Parameters of the Drude-Lorentz fit

| no. | $\omega_c$ ($cm^{-1}$) | $\omega_p$ ($cm^{-1}$) | $\gamma$ ($cm^{-1}$) |
|---|---|---|---|
| 1 | 0 | 10514.48 | 30068.55 |
| 2 | 0 | 3276.97 | 1483.96 |
| 3 | 192.88 | 3264.11 | 415.34 |
| 4 | 4686.18 | 1528.20 | 1647.44 |
| 5 | 5547.08 | 1717.51 | 1426.88 |
| 6 | 6211.36 | 1814.33 | 1087.76 |
| 7 | 6800.14 | 1935.12 | 949.09 |
| 8 | 7480.94 | 2368.06 | 858.47 |
| 9 | 8148.49 | 2623.72 | 1166.99 |
| 10 | 8483.29 | 1624.23 | 691.15 |
| 11 | 9102.31 | 2284.33 | 1261.51 |
| 12 | 9782.15 | 2763.17 | 1210.73 |
| 13 | 10439.48 | 1164.42 | 1182.40 |
| 14 | 11242.06 | 2436.71 | 1803.03 |
| 15 | 12264.05 | 2446.42 | 1957.35 |
| 16 | 13376.87 | 2351.99 | 1545.71 |
| 17 | 14544.81 | 2436.93 | 2017.53 |
| 18 | 15226.19 | 1933.59 | 1471.20 |
| 19 | 16565.46 | 2066.20 | 2049.04 |
| 20 | 17672.86 | 2436.53 | 2438.35 |
| 21 | 19356.83 | 1505.47 | 1711.46 |
| 22 | 20392.47 | 926.58 | 1957.04 |
| 23 | 21790.21 | 2091.53 | 2386.88 |
| 24 | 23964.34 | 1392.05 | 1893.15 |
| 25 | 26111.14 | 1399.13 | 1673.20 |
| 26 | 28435.61 | 1038.47 | 1465.94 |
| 27 | 30523.11 | 30056.74 | 63384.82 |
| 28 | 34846.75 | 3403.22 | 5855.71 |
| 29 | 36342.66 | 23077.90 | 21487.25 |
| 30 | 54718.26 | 8149.25 | 22536.52 |

$M_{00}$

$S_{11}$

$S_{22}$

$M_{11}$

$S_{33}$

Background

CG-3. Optical conductivity and the fitted oscillators

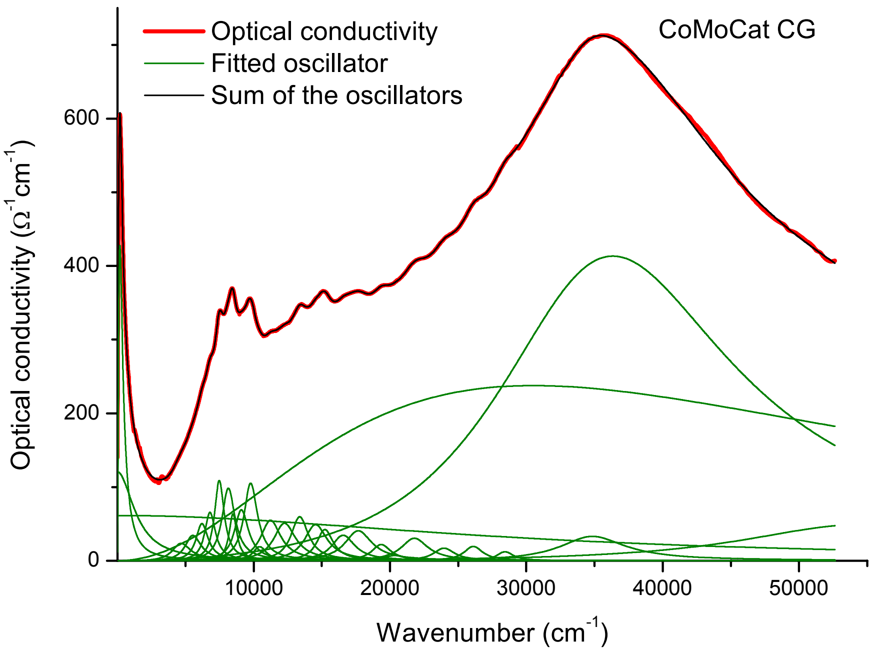


CG-4. The extracted $M_{00}$, $S_{11}$, $S_{22}$, $M_{11}$ peaks

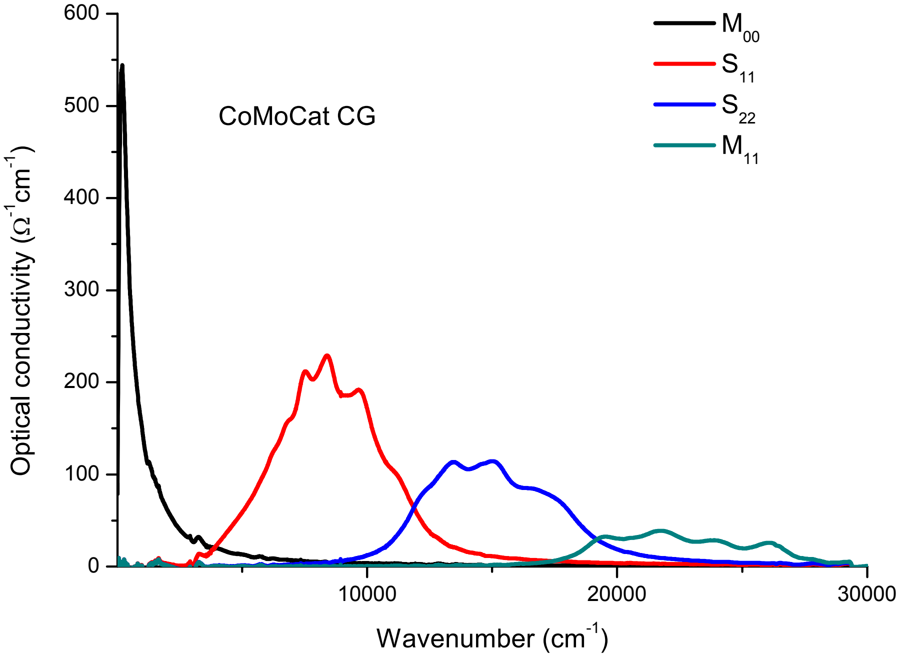

CG-5. The wavenumber ranges used in the diameter determination

| Wavenumber ranges for diameter determination | | | |
|---|---|---|---|
| Semiconducting | 6466 | - | 9550 |
| Metallic | 18501 | - | 26948 |

CG-6. Semiconducting and metallic nanotube species with transitions in the defined regions.

| $S_{11}$ (eV) | n | m | d (nm) |
|---|---|---|---|
| 1.241 | 7 | 3 | 0.706 |
| 1.219 | 7 | 5 | 0.829 |
| 1.194 | 11 | 0 | 0.873 |
| 1.192 | 8 | 1 | 0.678 |
| 1.177 | 10 | 2 | 0.884 |
| 1.130 | 9 | 4 | 0.916 |
| 1.113 | 8 | 4 | 0.840 |
| 1.112 | 7 | 6 | 0.895 |
| 1.095 | 9 | 2 | 0.806 |
| 1.083 | 10 | 0 | 0.794 |
| 1.064 | 8 | 6 | 0.966 |
| 1.062 | 12 | 1 | 0.995 |
| 1.039 | 11 | 3 | 1.014 |
| 0.996 | 9 | 5 | 0.976 |
| 0.996 | 10 | 5 | 1.050 |
| 0.995 | 10 | 3 | 0.936 |
| 0.989 | 11 | 1 | 0.916 |
| 0.983 | 8 | 7 | 1.032 |
| 0.951 | 13 | 2 | 1.120 |
| 0.942 | 9 | 7 | 1.103 |
| 0.926 | 12 | 4 | 1.145 |
| 0.903 | 12 | 2 | 1.041 |
| 0.903 | 11 | 4 | 1.068 |
| 0.902 | 13 | 0 | 1.032 |
| 0.896 | 10 | 6 | 1.111 |
| 0.889 | 11 | 6 | 1.186 |
| 0.879 | 9 | 8 | 1.170 |

| $M_{11}$ (eV) | n | m | d (nm) |
|---|---|---|---|
| 3.328 | 7 | 1 | 0.599 |
| 3.225 | 4 | 4 | 0.550 |
| 3.109 | 6 | 3 | 0.630 |
| 3.035 | 9 | 0 | 0.715 |
| 2.947 | 8 | 2 | 0.728 |
| 2.910 | 5 | 5 | 0.688 |
| 2.767 | 7 | 4 | 0.766 |
| 2.719 | 10 | 1 | 0.836 |
| 2.614 | 9 | 3 | 0.859 |
| 2.606 | 6 | 6 | 0.825 |
| 2.474 | 12 | 0 | 0.953 |
| 2.471 | 8 | 5 | 0.902 |
| 2.434 | 11 | 2 | 0.963 |

CG-7. The calculated average diameters

| average diameter (nm) | |
|---|---|
| semiconducting | 0.966 |
| metallic | 0.770 |
| overall | 0.902 |
| non armchair metallic | 0.795 |

CG-8.  The most abundant nanotubes in the sample

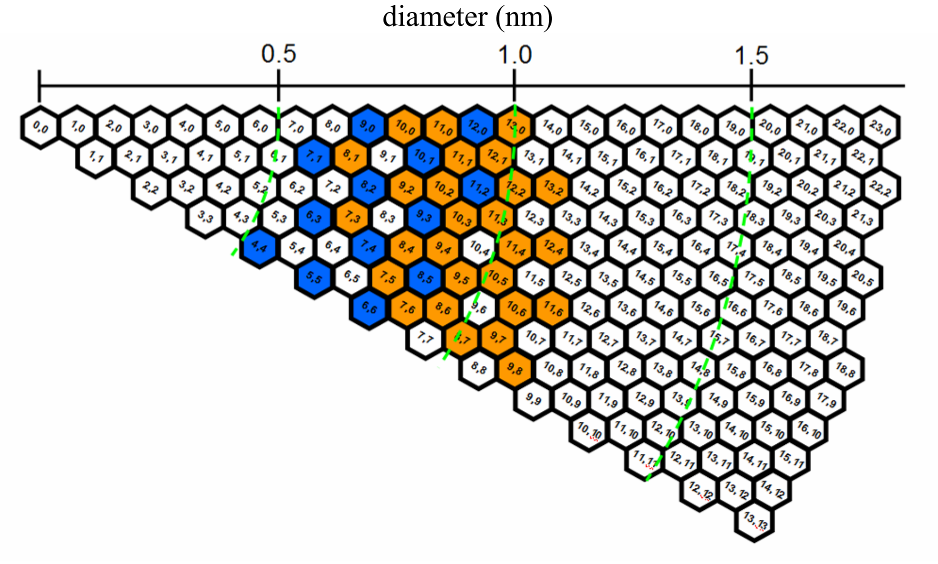


metallic and small-gap nanotube

semiconducting nanotube

# CoMoCat SG sample

SG-1. Transmission spectrum and optical conductivity

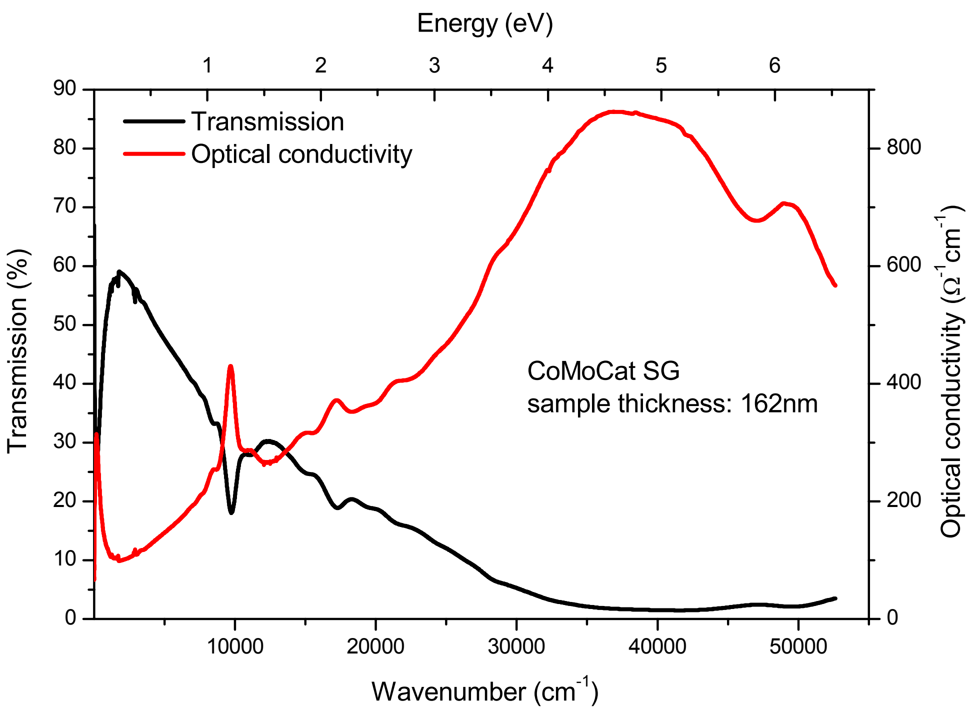


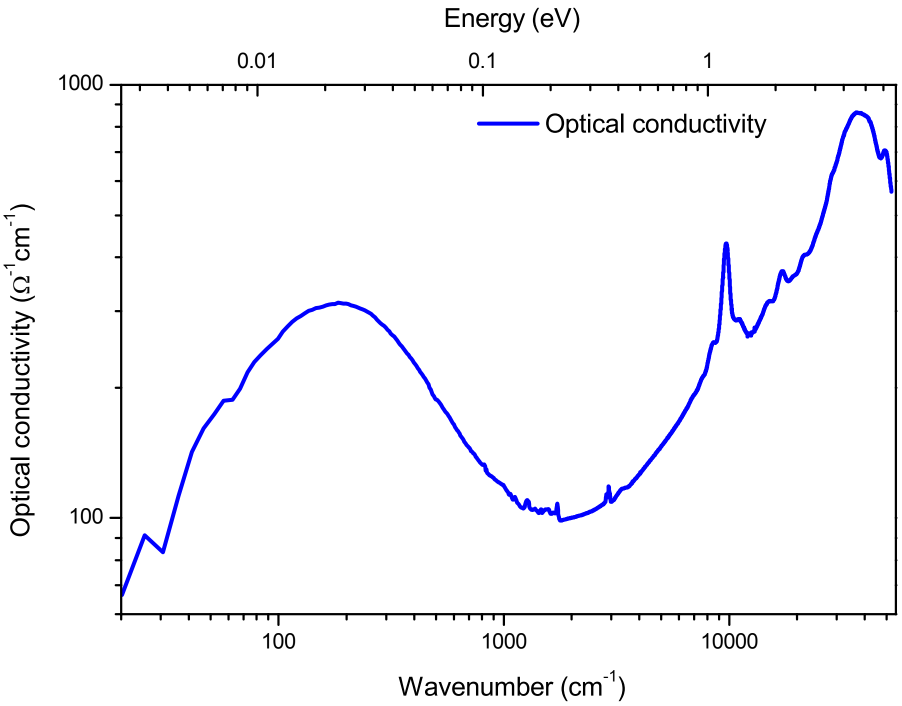

SG-2. Parameters of the Drude-Lorentz fit

| no. | $\omega_c$ ($cm^{-1}$) | $\omega_p$ ($cm^{-1}$) | $\gamma$ ($cm^{-1}$) |
|---|---|---|---|
| 1 | 0 | 8718.39 | 15924.77 |
| 2 | 0 | 107.99 | 133.83 |
| 3 | 179.91 | 2391.58 | 402.81 |
| 4 | 5994.56 | 3551.02 | 7373.83 |
| 5 | 6944.47 | 1098.18 | 1725.56 |
| 6 | 7564.00 | 477.47 | 503.59 |
| 7 | 8368.06 | 1382.74 | 860.67 |
| 8 | 9685.79 | 3379.72 | 887.10 |
| 9 | 11000.81 | 1118.91 | 933.34 |
| 10 | 11418.99 | 1255.05 | 1365.51 |
| 11 | 14158.72 | 1552.23 | 2418.67 |
| 12 | 14884.81 | 1146.02 | 1278.43 |
| 13 | 17103.11 | 2510.98 | 1773.45 |
| 14 | 19165.11 | 945.67 | 1395.26 |
| 15 | 21327.88 | 1747.21 | 1839.70 |
| 16 | 24275.66 | 994.77 | 1657.39 |
| 17 | 25119.54 | 27878.50 | 54911.73 |
| 18 | 26047.32 | 757.04 | 1839.26 |
| 19 | 28356.79 | 2031.25 | 2030.41 |
| 20 | 35352.83 | 23748.12 | 17542.52 |
| 21 | 42454.77 | 12259.19 | 10635.23 |
| 22 | 50232.19 | 10273.42 | 6643.31 |

$M_{00}$

$S_{11}$

$S_{22}$

$M_{11}$

$S_{33}$

Background

SG-3. Optical conductivity and the fitted oscillators

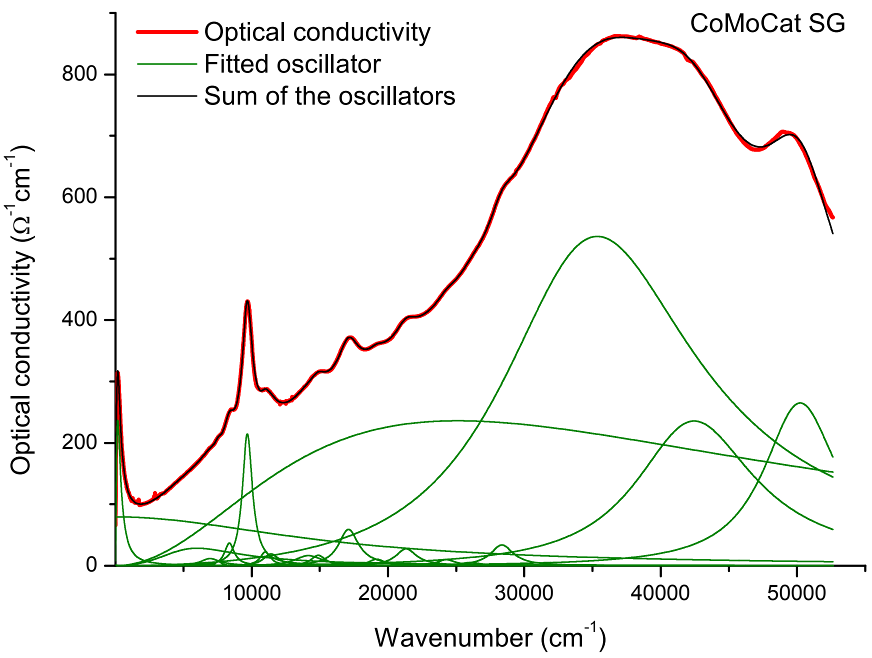


SG-4. The extracted $M_{00}$, $S_{11}$, $S_{22}$, $M_{11}$ peaks

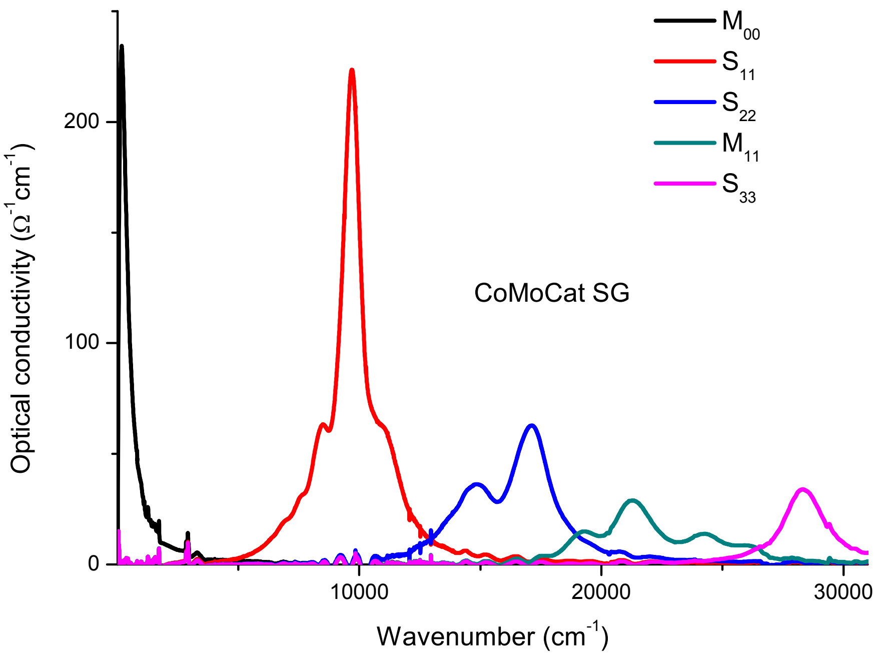

SG-5. The wavenumber ranges used in the diameter determination

| Wavenumber ranges for diameter determination | | | |
|---|---|---|---|
| Semiconducting | 8650 | - | 10303 |
| Metallic | 18468 | - | 26967 |

SG-6. Semiconducting and metallic nanotube species with transitions in the defined regions

| $S_{11}$ (eV) | n | m | d (nm) |
|---|---|---|---|
| 1.347 | 6 | 2 | 0.572 |
| 1.346 | 9 | 1 | 0.757 |
| 1.299 | 8 | 3 | 0.782 |
| 1.274 | 6 | 5 | 0.757 |
| 1.260 | 7 | 0 | 0.556 |
| 1.241 | 7 | 3 | 0.706 |
| 1.219 | 7 | 5 | 0.829 |
| 1.194 | 11 | 0 | 0.873 |
| 1.192 | 8 | 1 | 0.678 |
| 1.177 | 10 | 2 | 0.884 |

| $M_{11}$ (eV) | n | m | d (nm) |
|---|---|---|---|
| 3.328 | 7 | 1 | 0.599 |
| 3.225 | 4 | 4 | 0.550 |
| 3.109 | 6 | 3 | 0.630 |
| 3.035 | 9 | 0 | 0.715 |
| 2.947 | 8 | 2 | 0.728 |
| 2.910 | 5 | 5 | 0.688 |
| 2.767 | 7 | 4 | 0.766 |
| 2.719 | 10 | 1 | 0.836 |
| 2.614 | 9 | 3 | 0.859 |
| 2.606 | 6 | 6 | 0.825 |
| 2.474 | 12 | 0 | 0.953 |
| 2.471 | 8 | 5 | 0.902 |
| 2.434 | 11 | 2 | 0.963 |

SG-7. The calculated average diameters

| average diameter (nm) | |
|---|---|
| semiconducting | 0.739 |
| metallic | 0.770 |
| overall | 0.755 |
| non armchair metallic | 0.795 |

SG-8. The most abundant nanotubes in the sample

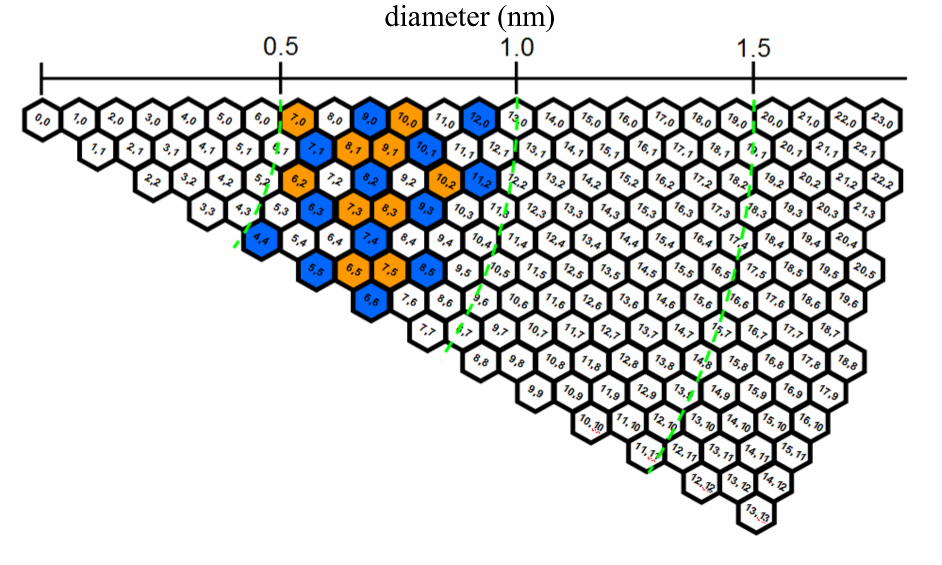


metallic and small-gap nanotube

semiconducting nanotube
